# Supplementary material for: How to predict community responses to perturbations in the face of imperfect knowledge and network complexity
Source: arXiv:1302.3757 source file (2013-09-16)
Supplement: Supplementary file 1 [file Supplement.pdf]

# Online Supplementary Material to: How to predict community responses to perturbations in the face of imperfect knowledge and network complexity

Helge Aufderheide,[1,2] Lars Rudolf,[2] Thilo Gross,[2] and Kevin D. Lafferty[3]
[1]*Max-Planck-Institute for the physics of complex systems, Dresden, Germany*
[2]*University of Bristol, Merchant Venturers School of Engineering, Bristol, UK*
[3]*U.S. Geological Survey, Western Ecological Research Center, Marine Science Institute, University of California, Santa Barbara, CA 93106*

**Contents**

**I. Review of the generalized modeling approach** 1

**II. Predator-prey example** 3

**III. Step-by-step parametrization of the Gatun Lake food web** 3
A. Parametrization 4
B. Estimation of the impact caused by the introduction of peacock bass 5

**IV. Derivation of influence and sensitivity** 6

**V. Model food webs** 7

**VI. Quality assessment of an impact prediction** 8

**VII. Figures for a higher food web connectance** 8

**References** 10

## I. REVIEW OF THE GENERALIZED MODELING APPROACH

In this section we first review the process of generalized modeling for food webs, which is presented more rigorously in Ref. 1. Further, we give the explicit expressions of the Jacobian matrix required for the perturbation impact evaluation in the paper.

The generalized model approach presented in Ref. 1 consists of four steps. First, a generalized model describes different food web populations $X_1, \ldots, X_N$. Depending on the application, the variable $X_i$ can describe species density, biomass abundance, carbon abundance or another characteristic quantity. Here, we assume that it denotes the total amount of biomass that can be attributed to a given species. The interactions and dynamics of the different populations $X_1, \ldots, X_N$ are described by $N$ differential equations of the form

$$\frac{\mathrm{d}}{\mathrm{dt}} X_i = G_i(X) + S_i(X_i) - L_i(X) - M_i(X_i), \tag{1}$$

where $G_i$, $L_i$, $M_i$, and $S_i$ are unspecified functions describing, respectively, the biomass gain by predation ($G_i$), the biomass loss by predation ($L_i$), the loss due to natural mortality ($M_i$), and the gain by primary production ($S_i$) of the focal species. We note that, while the primary production $S_i$ and the mortality $M_i$ only depend on the focal population $X_i$, the predatory gain $G_i$ and loss $L_i$ reflect the structure of the feeding relations in the food. Therefore $G_i$ and $L_i$ may depend on all other populations $X$. For instance, for a species $i$ with exactly one predator $j$, the loss through predation $L_i$ depends on the abundance of the species $X_i$, on the abundance of the predator $X_j$, and possibly on the abundances of other species that are also prey to $j$ due to apparent competition. However, $L_i$ does not depend directly on the abundances of the remaining species in the food web. Second, we assume that each species in this food web has a positive, yet unknown, abundance $X_i^* > 0$, i.e. all the species in the system coexist.

Mathematically this means, that $G_i, S_i, L_i, M_i$ are only reasonable modeling functions if the Jacobian matrix of the system (1) near $X^*$ has only negative eigenvalues (eigenvalues with negative real part) [3]. Generalized models facilitate finding such interaction functions $G_i, S_i, L_i, M_i$ through the two remaining steps.

Third, we formally establish the Jacobian matrix $\mathbf{J}$ for (1) for the unknown value of $X^*$ and for unknown functions $G_i, S_i, L_i, M_i$. Simply writing the necessary derivatives, the Jacobian matrix does not contain the functions $G_i, S_i, L_i, M_i$ directly, but only contains their partial derivatives, such as $\partial G_i/\partial X_i|_*$, where $|^*$ means that after taking the derivative by $X_j$ the values of $X^*$ should be inserted. For any given function $G_i$ and a given value of $X^*$ this derivative is a simple number. Finding suitable functions $G_i, L_i, M_i, S_i$ is therefore reduced to finding functions for which the partial derivatives at the steady state, e.g. $\partial G_i/\partial X_i|_*$, result in such values that the Jacobian matrix has only negative eigenvalues. Thus we can reinterpret the partial derivatives as parameters that describe the functional forms used in the model and study the stability of the Jacobian matrix in terms of their values.

Fourth, because the partial derivatives in the Jacobian matrix are hard to interpret directly and because they may depend on the (unknown) steady state, we write each of them in terms of intuitive parameters that can be measured in real-world systems. More precisely, we use the identity

$$\left.\frac{\partial G_i}{\partial X_i}\right|_* = \frac{G_i^*}{X_i^*} \left.\frac{\partial \log G_i}{\partial \log X_i}\right|_* , \tag{2}$$

which is true for $G_i(X^*), X_i^* > 0$ (a condition that is met for a system that is in a state of coexistence). This breaks each local derivative up into the product of two values. The first value, $\frac{G_i^*}{X_i^*}$, is the total per capita loss rate of species $i$ at the steady state. The second value, $\left.\frac{\partial \log G_i}{\partial \log X_i}\right|_*$, is a logarithmic derivative, also called elasticity. It measures the nonlinearity of $G_i$ at the steady state. For instance, for a power-law, $f(x) = Ax^p$, the logarithmic derivative is $\partial \log f/\partial \log x = p$, independently of $A$ or $x$. Or, if the gain by predation of a predator $i$ follows the well-known Holling type-II functional response $G_i \propto X_j/(1 + aX_j)$, then the logarithmic derivative of $G_i$ with regard to the prey abundance $X_j$ equals $1/(1 + aX_j^*)$, which is one for small prey abundances (linear increase of predation gain with prey abundance) and zero for very large prey abundances (predator is saturated with prey). Similar to $\left.\frac{\partial G_i}{\partial X_i}\right|_*$, the partial derivatives of $L_i, S_i$ and $M_i$ can be broken up into one per-capita rate of loss or gain and into one elasticity characterizing its nonlinearity at the steady state. In the following, the turnover rates and elasticities characterizing the partial derivatives are called generalized parameters.

In summary, for a given food web, choosing a combination of the generalized parameters is equivalent to choosing specific values for the partial derivatives in the Jacobian matrix, and thus to choosing the properties of the model functions $G_i, L_i, M_i, S_i$ near the steady state. Characterizing those combinations of parameters that lead to a Jacobian matrix with only negative eigenvalues is therefore equivalent to finding food web models that allow a stable steady state on the given food web topology.

For the generalized model for food webs presented in Ref. 1, the generalized parameters resulting from the described procedure are given in Tab. I (see main article). Further, the diagonal and off-diagonal entries of the Jacobian matrix in terms of these generalized parameters are then given by [1]

$$\begin{aligned} J_{ii} = \alpha_i \Bigg( & \tilde{\rho}_i \Phi_i + \rho_i \left(\gamma_i \chi_{ii} \lambda_{ii} + \Psi_i\right) \\ & - \tilde{\sigma}_i \mu_i - \sigma_i \left( \sum_k \beta_{ki} \lambda_{kj} \left((\gamma_k - 1)\chi_{ki} + 1\right)\right)\Bigg) \\ J_{ij} = \alpha_i \Bigg( & \rho_i \gamma_i \chi_{ij} \lambda_{ij} \\ & - \sigma_i \left( \beta_{ji} + \sum_k \beta_{ki} \lambda_{kj} \left((\gamma_k - 1)\chi_{k,j}\right)\right)\Bigg), \end{aligned}$$

where $\tilde{\rho} = 1 - \rho$ and $\tilde{\sigma} = 1 - \sigma$.

Intuitively, the terms in the first line of each expression result from biomass intake, either from primary production $S_i$ of the focal species $i$ ($\rho_i = 0$ for primary producers) or through the predation gain $G_i$ from species $j$ ($\rho_i = 1, \chi_{ij} \neq 0$ if $i$ predates on $j$). The expressions in the second line of each expression result from to the loss of the focal species $i$, either from natural mortality $M_i$ of the focal species $i$ ($\tilde{\sigma}_i > 0$) or through the predation loss $L_i$ caused by species $j$ ($\sigma_i > 0$, $\beta_{j,i} \neq 0$ if $j$ predates on $i$). The sums over $k$ hereby result from the effects of apparent competition if $i$ and $j$ share a common predator $k$, because the predation of $k$ changes when more prey is available. A more detailed discussion is given in Ref. 1.

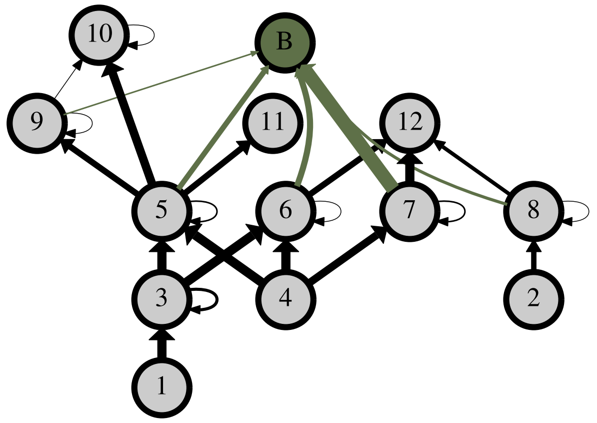


1 Nanophytoplankton
2 Filamentous green algae
3 Zooplankton
4 Insects
5 Silverside (Melaniris chagresi)
6 Tetras (Characidae)
7 Sailfin Molly/Mosquito Fish (Poeciliidae)
8 Blackbelt Cichlid (Cichlasoma maculicauda)
9 Bigmouth Sleeper (Gobiomorus dormitor)
10 Tarpon (Tarpon atlanticus)
11 Black Tern (Chlidonias niger)
12 Herons and Kingfishers
B Peacock Bass (Cichla ocellaris)
5–11, and B are species,
1–4 and 13 are aggregated taxa.

FIG. 1: Food Web description of the Gatun Lake ecosystem [4]. Each species or aggregated taxon is marked by a node, the feeding interactions between the species as edges. Edges from a node to itself mark cannibalistic interactions, commonly encountered by the fish species feeding on younger individuals of their own species. Numbered species and black (solid) edges indicated the established ecosystem. Bold edges represent feeding links from a predator's principle food source. Colored edges mark the feeding interactions of the introduced peacock bass populations.

## II. PREDATOR-PREY EXAMPLE

In this appendix we provide the explicit calculations of the perturbation impact for the simple producer-grazer example. In this system, a grazer of biomass density $X_1$ consumes a primary producer of biomass density $X_2$. The Jacobian matrix near the steady state is then (see Sec. I)

$$\mathbf{J} = \begin{pmatrix} \alpha_1(\psi_1 - \mu_1) & \alpha_1\gamma_1 \\ -\alpha_2\sigma_2\psi_1 & \alpha_2(\phi_2 - \sigma_2\gamma_2 - \tilde{\sigma}_2\mu_2) \end{pmatrix}.$$

A discussion of stability of this system in terms of the generalized modeling parameters can be found in Refs. 1, 2.

For calculating the impact of a given perturbation for each of the two species, we require the inverse of the Jacobian

$$\mathbf{J}^{-1} = \frac{1}{\det \mathbf{J}} \begin{pmatrix} \alpha_2(\phi_2 - \sigma_2\gamma_2 - \tilde{\sigma}_2\mu_2) & -\alpha_1\gamma_1 \\ \alpha_2\sigma_2\psi_1 & \alpha_1(\psi_1 - \mu_1) \end{pmatrix},$$

where

$$\det \mathbf{J} = \alpha_1\alpha_2(\phi_2 - \sigma_2\gamma_2 - \tilde{\sigma}_2\mu_2 + \sigma_2\gamma_1\psi_1)(\psi_1 - \mu_1)$$

denotes the determinant of $\mathbf{J}$.

As a perturbation, we now consider a new grazer that has a direct negative effect on the primary producer, but no direct effect on the established grazer. The perturbation $K$ is therefore given by $K_1 = 0$, $K_2 < 0$. Now we plug this vector $K$ in the impact equation to obtain $I = -\mathbf{J}^{-1}(0, K_2)^T$. The impact on the grazer,$I_1$, and the impact on the producer, $I_2$, are therefore

$$I_1 = \frac{\alpha_1}{\det \mathbf{J}}\gamma_1 K_2 \quad \text{and} \quad I_2 = \frac{\alpha_1}{\det \mathbf{J}}(\mu_1 - \psi_1)K_2.$$

## III. STEP-BY-STEP PARAMETRIZATION OF THE GATUN LAKE FOOD WEB

Here we apply the generalized model approach to parametrize the real-world food web of Gatun Lake in Panama [4] shown in Fig. 1. The intention of this example is to demonstrate the method described in the paper and give a more hands-on approach towards such a parametrization. To keep the parametrization process clear, we therefore choose a very simplistic parametrization. After the parametrization, we analyze the perturbation consequences of an invasion of this food web by the predatory peacock bass *Cichla ocellaris*, as described in 4. We note that the process of parametrization and computation of the perturbation impact on this food web was done using the program code provided as online supplement to this paper [5, 6].

| Species | | Generalized Parameters | | | | Other Parameters | | |
|---|---|---|---|---|---|---|---|---|
| $i$ | Name | $\alpha_i$ | $\rho_i$ | $\sigma_i$ | $\chi_{ii}$ | $\beta_{ii}$ | $M_i$ (g) | $\chi_{Bi}$ |
| 1 | Nanophytoplankton | 203.3 | 0 | 0.62 | - | - | $10^{-6}$ | - |
| 2 | Filamentous green algae | 30 | 0 | 0.50 | - | - | 0.0003 | - |
| 3 | Zooplankton | 30 | 1 | 0.9 | 0.25 | 0.32 | 0.002 | - |
| 4 | Insects (mosquitoes) | 5 | 0 | 0.82 | - | - | 0.003 | - |
| 5 | Silverside | 2.509 | 1 | 0.80 | 0.09 | 0.11 | 5.2 | 0.30 |
| 6 | Tetras | 1.432 | 1 | 0.59 | 0.08 | 0.13 | 49 | 0.17 |
| 7 | Sailfin M.&Mosquito F. | 3.89 | 1 | 0.66 | 0.20 | 0.30 | 0.89 | 0.39 |
| 8 | Blackbelt Cichlid | 0.847 | 1 | 0.49 | 0.18 | 0.37 | 400 | 0.09 |
| 9 | Bigmouth Sleeper | 0.38 | 1 | 0.26 | 0.14 | 0.56 | 1716 | 0.05 |
| 10 | Tarpon | 0.33 | 1 | 0.13 | 0.08 | 1 | 24000 | - |
| 11 | Black Tern | 1.39 | 1 | 0 | - | - | 55 | - |
| 12 | Herons and Kingfishers | 0.71 | 1 | 0 | - | - | 800 | - |
| B | Peacock bass | 0.64 | - | - | - | - | 1213 | - |

| Spec. | | Gen. Param. | |
|---|---|---|---|
| $i$ | $j$ | $\chi_{ji}$ | $\beta_{ji}$ |
| 1 | 3 | 1 | 1 |
| 2 | 8 | 0.82 | 1 |
| 3 | 5 | 0.46 | 0.91 |
| 3 | 6 | 0.46 | 0.08 |
| 4 | 5 | 0.45 | 0.74 |
| 4 | 6 | 0.47 | 0.07 |
| 4 | 7 | 0.80 | 0.19 |
| 5 | 9 | 0.86 | 0.31 |
| 5 | 10 | 0.83 | 0.40 |
| 5 | 11 | 1 | 0.18 |
| 6 | 12 | 0.33 | 0.87 |
| 7 | 12 | 0.46 | 0.69 |
| 8 | 12 | 0.21 | 0.63 |
| 9 | 10 | 0.09 | 0.50 |

TABLE I: Modeling Parameters estimated for the Gatun Lake food web. $\alpha_i$, $\psi_i$, $\rho_i$, $\sigma_i$, $\chi_{ij}$ and $\beta_{ij}$ are generalized parameters as used throughout the paper. All other generalized parameters are identical for all species, i.e. $\gamma = 0.95, \phi = 0.5, \lambda = 1, \mu = 1, \psi_{fish} = 1, \psi_{bird} = 1.02, m_i = 0.12$. $M_i$ is the used typical body mass of individuals from each species, and $\chi_{Bi}$is the relative diet composition the peacock bass.

### A. Parametrization

For a given food web, the generalized model presented in Sec. I describes a broad class of different food web models. Testing a given model in this class through numerical computations requires setting all parameters $\alpha, \gamma, \mu, \phi, \psi, \beta, \chi, \sigma, \rho$ to specific values, i.e. we have to parametrize the model. In our example parametrization, the parameters $\alpha, \gamma, \mu, \phi, \psi$ are chosen independently from the underlying food web topology, while the remaining parameters $\chi, \beta, \sigma, \rho$ depend on the strength of the feeding relations between the different species.

The parameters used in our model are set using the following rules. The resulting parameters are given explicitly in Tab. I.

- $\alpha_i = (0.00485\, M_i)^{-1/4}$. The species turnover rates are scaled allometrically with their body mass $M_i$, unless more precise explicit empirical knowledge is available. The pre-factor 0.00485 was determined by the best fit of available turnover data.

- $\mu_i = 1$. The loss of biomass through natural mortality of each species increases linearly with the species' abundance.

- $\psi_i = 1$ for fish and 1.02 for birds. The predation gain increases linearly with the abundance of fish. For birds the predation gain increases slightly faster because increasing bird abundance decreases the fish refugium from predation.

- $\phi_i = 0.5$. The biomass gain of primary producer species' in the food web increases sublinearly with the primary producer's abundance, because of space or nutrient constraints.

- $\gamma_i = 0.95$. The biomass gain through predation of a predator species increases slightly slower than the abundance of its prey. Intuitively, this is due to a saturation in prey of the predator as in the well-known Holling type-II functional response.

- $\lambda_{ij} = 1$. All prey switching coefficients are equal. The value 1 indicates, that a predator has no dietary preferences and switches passively between different prey species.

- $\rho_i = 0$ for primary producers and $\rho_i = 1$ for predators. Each species gains biomass either by primary production or by predation, but not both.

- $\chi_{ji}$ reflects the relative contribution of species $i$ to species $j$'s diet. To parametrize this, we use allometric relationships between consumer and prey body sizes. More precisely, we estimate for each predator the preferred

| Species | | Observed | Impact |
|---|---|---|---|
| No. | Name | change [4] | $I_B/\kappa$ |
| 1 | Nanophytoplankton | decrease | -0.06 |
| 2 | Filamentous green algae | ? | +0.06 |
| 3 | Zooplankton | increase | +0.05 |
| 4 | Insects (Mosquitoes) | increase | +0.04 |
| 5 | Silverside | -50% | -0.6 |
| 6 | Tetras | -95% | -0.3 |
| 7 | Sailfin Molly &Mosquito Fish | -100% | +0.24 |
| 8 | Blackbelt Cichlid | +50% | -0.06 |
| 9 | Bigmouth Sleeper | -90% | -0.16 |
| 10 | Tarpon | decrease | -1.25 |
| 11 | Black Tern | decrease | +3 |
| 12 | Herons and Kingfishers | decrease | -0.1 |

TABLE II: Comparison of the observed long-term changes in the species abundances after the introduction of the peacock bass [4] with the assessed impact of the perturbation corresponding to this introduction. For the impact $I_B$ represents the response to the population of peacock bass.

prey body mass and a typical prey body mass range from Table 1 in Ref. [7], individually considering allometric scaling for birds, fishes, and invertebrate predators. Then, we consider that for each predator with a preferred prey body mass $\mathrm{M_{pref}}$ the feeding on prey with a body mass $\mathrm{M_{prey}}$ is distributed normally with $\log(\mathrm{M_{prey}}/\mathrm{M_{pref}})$, where the width of the normal distribution is estimated from the typical prey body mass range of each consumer. Thus we obtain for each predator-prey relation in the food web the preference $e_{ki}$ of the predator $k$ to consume the prey $i$. To obtain $\chi_{ki}$, we normalize these contributions, i.e. $\chi_{ki} = e_{ki}/\sum_j e_{kj}$.

- $\sigma_i$, indicating biomass loss due to predation relative to the total loss, strongly increases with predation pressure on a species. Using the feeding preferences established for $\chi$, we set $\sigma_i = \sum_k e_{ki}/(\sum_k e_{ki} + m_i)$, where $m_i$ is a measure for the importance of the loss through mortality relative to the feeding pressure measured by $\sum_k e_{ki}$.

- $\beta_{ji}$ represents the relative loss of a species $i$ to its different predators $j$. However, in general this predation loss of a species to different predators is not independent from the predation gain of the respective predators. In other words, the parameters $\beta$ are dependent on $\chi$. To resolve this dependency consistently, we assume that when a predator kills a prey, it consumes all its biomass, such that biomass is conserved throughout the process. We denote the total biomass loss rate of a species $i$ as $B_i$. For top predators, this loss is due only to natural mortality and we set $B_i = 1$. For all other species the conservation of biomass implies that the loss $B_i$ equals the intake of its predators, i.e. $B_i = \sum \chi_{ji} B_j/\sigma_j$, where $j$ runs over all of $i$'s predators. This system of linear equations can be solved for all the species biomass outflows $B$. Then the parameters $\beta$ are the contributions of each predator $j$ to the total loss of $i$, i.e. $\beta_{ji} = (\chi_{ji}/B_i)\, B_j/\sigma_j$.

This configuration of parameters is included as an example in our online code [5].

Once we have established the parametrization, we can write the Jacobian matrix $\mathbf{J}$ using the expressions given in Sec. I. Stability of any particular steady state (corresponding to a particular set of generalized parameters) is ensured by checking that all eigenvalues of the Jacobian have negative real parts [3]. For the Gatun Lake Food Web with the parametrization above, the eigenvalues with the largest real parts are the pair of complex conjugate eigenvalues $\lambda_\pm \approx -0.001 \pm 0.02\mathrm{i}$. Therefore, the chosen parametrization indeed corresponds to a steady state of coexisting species.

### B. Estimation of the impact caused by the introduction of peacock bass

Now, we compute the impact of a perturbation to the Gatun Lake food web. More specifically, we estimate the initial effect of the invasion of the lake by a predatory fish, such as the peacock bass, as described in Ref. 4.

We consider the increase of predation pressure on species that are prey to the peacock bass as the main direct perturbation of the established ecosystem. To quantify this perturbation for the different established species $i$ we now estimate the effect of the additional population of peacock bass $Y_B$. The perturbation of species $i$ due to increased

predation by $B$ is

$$K_{iB} = -\left.\partial L_i/\partial Y_B\right|_* = -\alpha_B \chi_{Bi} \kappa_i, \tag{3}$$

where we used (2) to split the derivative into the turnover rate $\alpha_B \chi_{Bi}$ ($\alpha_B$ is the turnover rate of the peacock bass and $\chi_{Bi}$ the relative contribution of $i$ to $B$'s diet), and an elasticity $\kappa_i = \partial \log L_i / \partial \log Y_B$. For simplicity, we assume in the following that $\kappa$ is identical for all species $i$ and therefore drop the corresponding index.

The peacock bass feeds on the secondary consumer fishes (tetras, silverside, and sailfin molly/mosquito fish, black-belt cichlid), and on the bigmouth sleeper [4]. To obtain the relative contributions of each of these species to its diet, $\chi_{ai}$, we employ the allometric scaling rules introduced to estimate the diets of species in the food web. This leads to the values indicated in Tab. I.

Plugging $\mathbf{J}$ and the perturbation for the peacock bass $\mathbf{K}$ into $\mathbf{I} = -\mathbf{J}^{-1}\mathbf{K}$ we obtain the ultimate impact of the perturbation shown in Fig. 1 of the paper. This computation can be easily done using our supplementary online code [6]. The resulting response (Fig. 2m) is given explicitly in Tab. II alongside the observed changes [4].

In addition to the perturbation caused by the peacock bass (Fig. 2m), we also consider the perturbation of the system due to a specialist predator feeding on only one species $i$, i.e. the diet of the predator (P) is characterized by $\chi_{P,i} = 1$. We observe, that the response to these perturbations (Fig. 2a-l) agrees well with the predicted sensitivity and influence (Fig. 2n,o). If an influential species is perturbed, generally all species show a strong response (e.g. Fig. 2k), but when a species with low influence is perturbed, generally only few species are strongly affected (e.g. Fig. 2b). Further, sensitive species generally respond strongly to perturbations elsewhere (e.g. species 6), while species with low sensitivity (e.g. species 5) show generally smaller responses.

## IV. DERIVATION OF INFLUENCE AND SENSITIVITY

Here, we derive the expressions for the influence and sensitivity of the food web species that are motivated in the paper with intuitive arguments. For this, we decompose the Jacobian matrix into the dynamical modes of the system. Then we use the impact-definition to identify sensitive species as those for which the expected impact of randomly excited modes is largest, and to identify influential species as those for which the expected excitation of dynamical modes is largest when they are perturbed.

The inverse Jacobian matrix $\mathbf{J}^{-1}$, required for the impact calculation, has the same right eigenvectors $v^{(k)}$ and left eigenvectors $w^{(k)}$ as the Jacobian matrix. Each pair $v^{(k)}, w^{(k)}$ correspond to the eigenvalue $1/\lambda_k$, where $\lambda_k$ is the eigenvalue of $\mathbf{J}$. Therefore, for a perturbation $K$, the impact equation $I = -\mathbf{J}^{-1}K$ can be written as the sum over the eigenvectors and eigenvalues of $\mathbf{J}$ as

$$I = \sum_k v^{(k)} \frac{w^{(k)} \cdot K}{-\lambda_k},$$

where $k$ runs over all eigenvalues and where $\cdot$ denotes the scalar product.

We see that for a given mode $k$ the contribution to the impact on a given node depends on three factors. First, the product $w^{(k)} \cdot K$ determines which dynamical modes are excited by the perturbation. Second, $v^{(k)}$ determines which entries in $I$ are affected by this dynamical mode. And finally, the excitability $1/\lambda_k$ indicates how strongly the mode will be excited.

For the sensitivity of a species, we do not want to explicitly refer to any particular perturbation $K$. In absence of additional information, we therefore consider the case of a perturbation affecting every dynamical mode $k$ with identical probability. The sensitivity $Se_i$ can thus be measured as the effects on node $i$,

$$\mathrm{Se}_i = \log\left(\sum_k \frac{\left|v^{(k)}{}_i\right|}{-\lambda_k}\right),$$

where $\left|v^{(k)}{}_i\right|$ denotes the absolute value of $v^{(k)}$ on node $i$, and where we used the logarithm to bring the numerical values into a more manageable range.

For the influence of a species, we evaluate the impact of a perturbation affecting only this specific species $K$. In absence of additional information, the influence is measured by the resulting excitation of all the dynamical modes

$$\mathrm{In}_i = \log\left(\sum_k \frac{\left|w^{(k)}{}_i\right|}{-\lambda_k}\right).$$

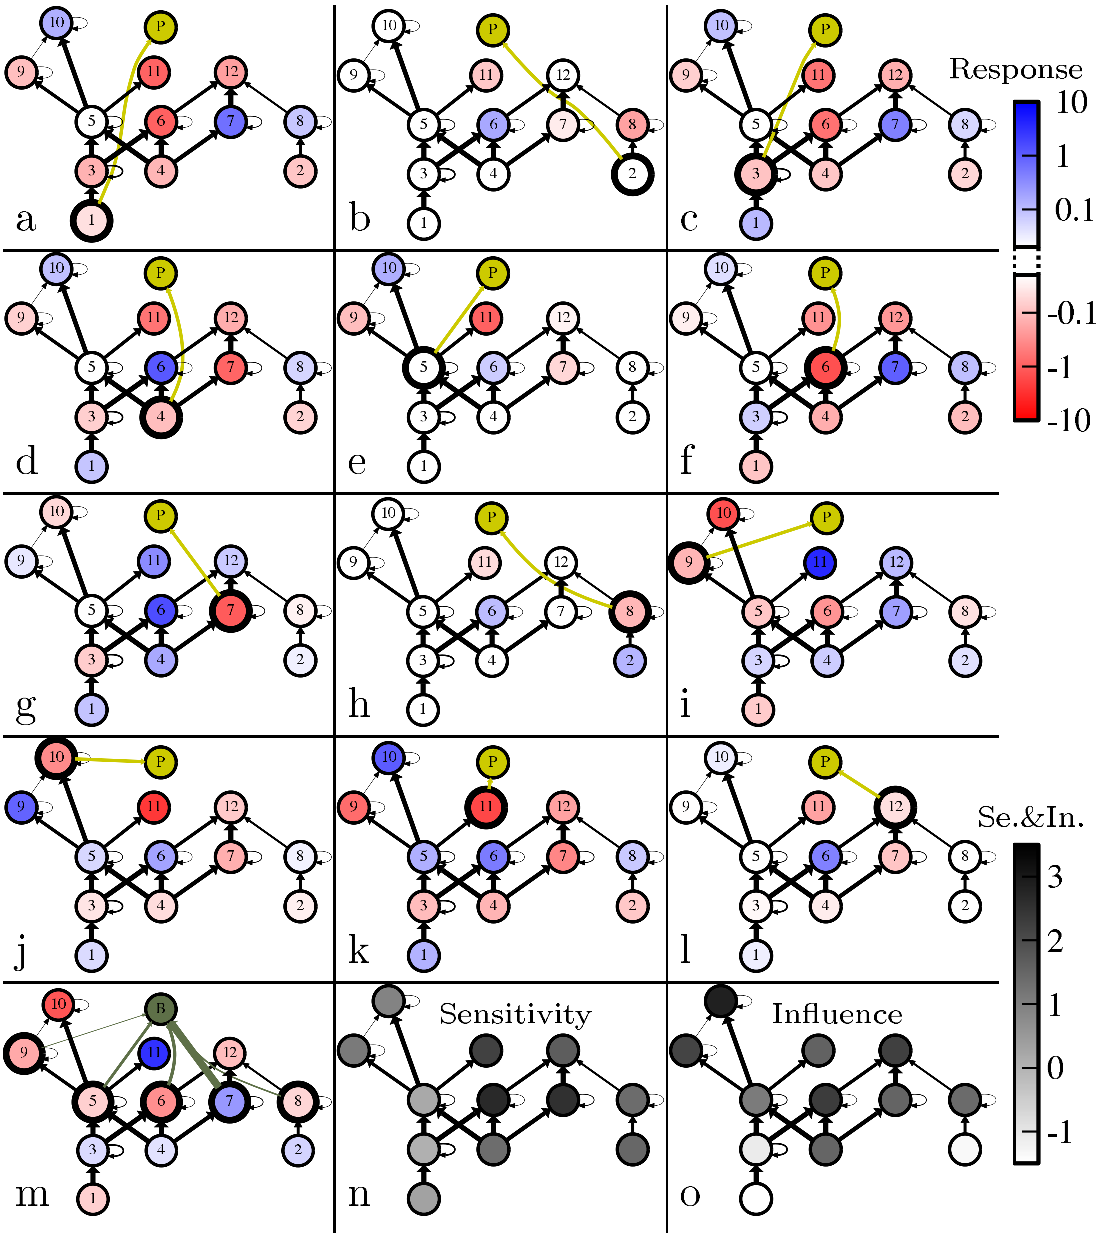


FIG. 2: Predicted response of the Gatun Lake food web [4] to different perturbations. Shown are species (circles) and predator-prey relationships (arrows, in the direction of the biomass flow). In each panel a-l) a different population is affected by a hypothetical specialized predator (P), such that the abundance of this species decreases. Panel m) shows the perturbation caused by the peacock bass (B). The color code denotes the response of each species to the different perturbations. In panels n) and o) the gray-scale denotes the sensitivity and the influence of each species respectively. Color online.

## V. MODEL FOOD WEBS

For the numerical experiments in our paper, we generate model food webs as suggested in Ref. 8. This process consists of two steps, topology generation and parametrization, which can be reproduced using our supplementary online code [5].

To generate the food web topology, we use the niche web algorithm [9]. This algorithm establishes a topology by assigning to each species a so-called niche value, denoting a species fitness or body size. Further it assigns to each species a range of niche values, called feeding range. If a species has a niche value that lies inside the feeding range of another species, then it is prey to this species.

Formally, the niche value $n_i$ of species $i$ is drawn from a uniform distribution between 0 and 1. Further, the

feeding range of viable prey niche values is given by $c_i - r_i/2 \dots c_i + r_i/2$, where $r_i$ denotes its size and $c_i$ its center. $r_i$ is obtained for each species by independently drawing a beta distribution variable (between 0 and 1) and then multiplying with the species' niche value $n_i$. The center value $c_i$ of this range, is then drawn uniformly between $r_i/2$ and $n_i$. We note, that this makes cannibalistic links possible, because $c_i - r_i/2 \dots c_i + r_i/2$, contains the niche value $n_i$, if $c_i > n_i - r_i/2$.

In our simulations, we use only niche model food webs meeting two requirements. First, topologies have to be connected, such that the resulting food web does indeed contain the desired number of species and does not separate into multiple smaller food webs. Second, the connectance of a generated food web cannot deviate more than 5% from the desired value.

After the topology of a food web is established, we parametrize the generated food web topology using the generalized model reviewed in Sec. I [1] . In other words, we sample a specific food web model for the given topology by drawing a set of specific values for the generalized parameters. For this sampling, species turnover rates $\alpha_i$ are set using allometric scaling with body mass, where the niche values are used as an indicator for their body size. All other parameters are sampled uniformly and independently from the ranges indicated in Tab. I in the main paper, for the parameters $\chi$ and $\beta$, the conditions $\sum_i \chi_{ij} = 1$ and $\sum_j \beta_{ij} = 1$ are enforced by subsequent normalization.

Once the food web is parametrized with a specific set of parameters, we can compute the Jacobian matrix and thus the stability of the chosen configuration. In our numerical experiments, we retain only configurations, that allow for a stable coexistence of species, i.e. configurations for which the largest Jacobian matrix eigenvalue has a negative real part.

## VI. QUALITY ASSESSMENT OF AN IMPACT PREDICTION

To assess the quality of an impact estimation, we compare the true impact $I$ computed using the true Jacobian matrix with the estimated impact $\tilde{I}$ computed using the estimated Jacobian matrix. The quality $Q$ of the impact estimation is evaluated as the cosine of the angle between the true and the estimated impact vector. Mathematically,

$$Q = \cos\left(I \angle \tilde{I}\right) = \frac{I \cdot \tilde{I}}{||I||\,||\tilde{I}||},$$

where $\cdot$ denotes the scalar product and $||I||$ is the norm of the vector $I$.

For instance, if $I = \tilde{I}$, i.e. if the estimation is exactly correct, then $Q = I \cdot I/||I||^2 = 1$. Further, if $I = -\tilde{I}$, i.e. if the estimation is exactly the opposite of the true impact, then $Q = -I \cdot I/||I||^2 = -1$.

## VII. FIGURES FOR A HIGHER FOOD WEB CONNECTANCE

Throughout the paper, we show graphs and results for for model food webs with a connectance of $C = 0.04$. Because of the great importance of the connectance for food web properties, for example for the stability of a food webs [8], we show here the same results based on model food webs with twice the connectance, i.e. for $C = 0.08$. The detailed description of the shown quantities and the interpretations of the graphs are given in the main paper. All of the following graphs have the same parameters as in the paper.

The impact as a function of importance and sensitivity is virtually identical to the results for $C = 0.04$ (Fig. 3). Close inspection reveals a slight increase in the overall values of importance and sensitivity.

The increase in prediction quality with iterative parameter estimation is qualitatively identical to the results for $C = 0.04$ (Fig. 4), but the overall quality of the prediction decreases.

The decrease of prediction quality with an error in one species property is qualitatively identical to the results for $C = 0.04$ (Fig. 5). The decrease with parameters referring to dietary preferences $\chi, \beta$ is more pronounced.

The correlations of sensitivity and influence with several species properties (Fig. 6) are similar to those found for $C = 0.04$. A significant increase is observed for the negative correlation between sensitivity and species vulnerability.

In summary, we observe that doubling the connectance generally has only a quantitative, but not qualitative effect on our results.

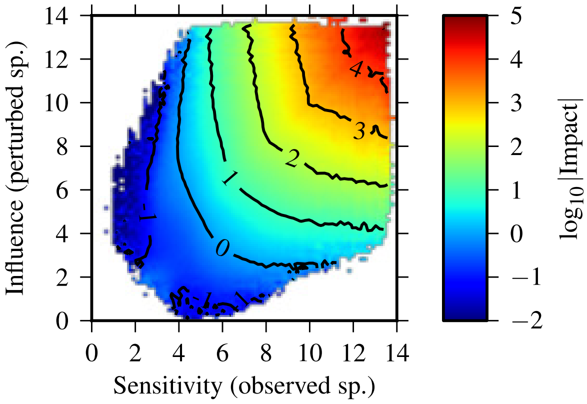


FIG. 3: The average absolute impact on a species with given sensitivity if a species of given influence is perturbed. See Fig. 2 in the main paper for details. Parameters: $N = 50$, $C = 0.08$.

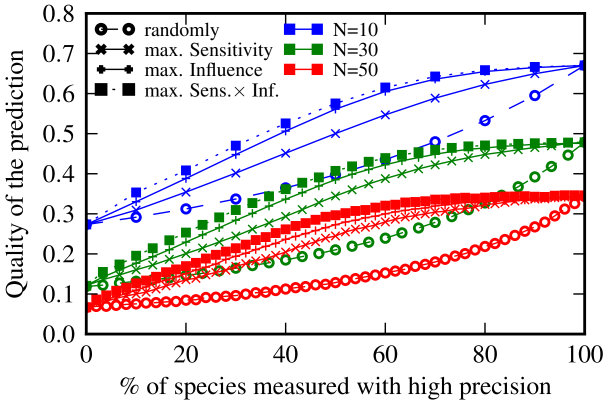


FIG. 4: Focusing on sensitive and important species can reduce the measurement effort when species are measured successively with higher precision. See Fig. 3 in the main paper for details. Parameters: $C = 0.08$.

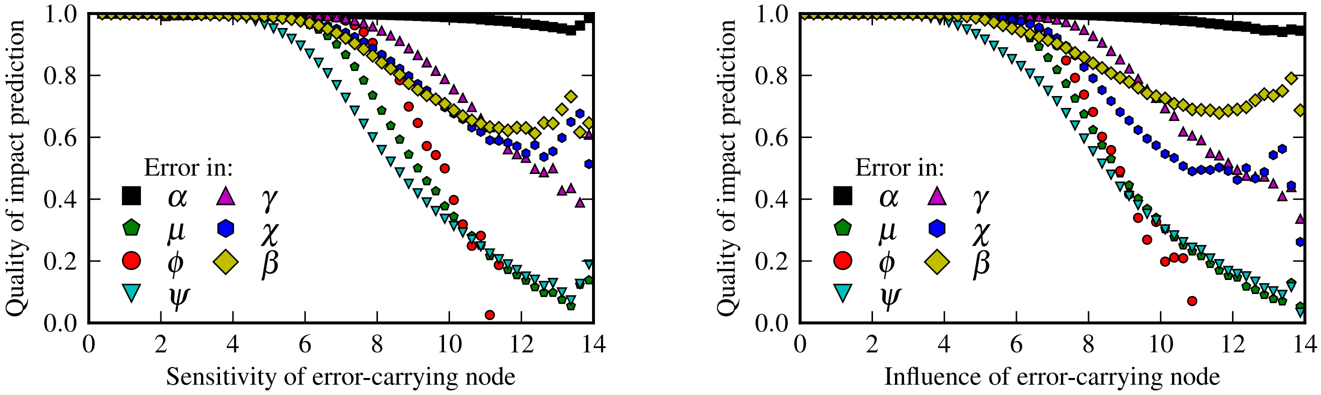


FIG. 5: Average quality of an impact prediction in the presence of measurement errors. The average quality of an impact prediction if one node with the specified sensitivity (left) or influence (right) in a food web is subject to a measurement error. See Fig. 4 in the main paper for details. Parameters: $N = 50$, $C = 0.08$.

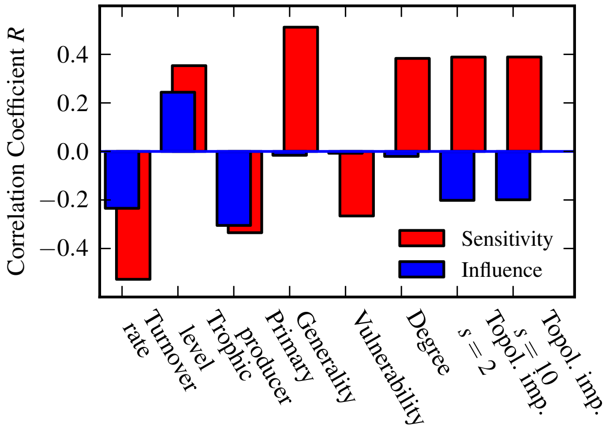


FIG. 6: Correlations of species' properties with their sensitivity and influence. See Fig. 5 in the main paper for details. Parameters: $N = 50$, $C = 0.08$.

[1] Thilo Gross and Ulrike Feudel. Generalized models as a universal approach to the analysis of nonlinear dynamical systems. *Phys. Rev. E*, 73(1):16205, 2006.
[2] Thilo Gross, Wolfgang Ebenhöh, and Ulrike Feudel. Enrichment and foodchain stability: the impact of different forms of predator–prey interaction. *Journal of Theoretical Biology*, 227(3):349–358, April 2004.
[3] Yuri A. Kuznétsòv. *Elements of applied bifurcation theory*, volume 112 of *Applied Mathematical Sciences*. Springer Verlag, 1998.
[4] Thomas M. Zaret and R. T. Paine. Species introduction in a tropical lake: A newly introduced piscivore can produce population changes in a wide range of trophic levels. *Science*, 182(4111):449–455, February 1973.
[5] Helge Aufderheide. Supplementary Code: Parametrizer for generalized models of food webs, May 2013. *www.biond.org/content/programming-tools* or *www.upontheheath.de/index.php/research/downloads-online-material*
[6] Helge Aufderheide. Supplementary Code: CIP - calculator for the impact of perturbations, January 2013. *www.biond.org/content/programming-tools* or *www.upontheheath.de/index.php/research/downloads-online-material*
[7] Ulrich Brose, Tomas Jonson, Eric L. Berlow Philip Warren et al. Consumer-resource body-size relationships in natural food webs. *Ecology*, 87(10):2411–2417, 2006.
[8] Thilo Gross, Lars Rudolf, Simon A. Levin, and Ulf Dieckmann. Generalized models reveal stabilizing factors in food webs. *Science*, 325(5941):747–750, 2009.
[9] Richard J. Williams and Neo D. Martinez. Simple rules yield complex food webs. *Nature*, 404(6774):180–183, 2000.
